# Supplementary material for: Forces and fluctuations in planar, spherical and tubular membranes
Source: arXiv:1011.1640 source file (2010-11-07)
Supplement: Supplementary file 1 [file appendix31.tex]

\chapter{Theoretical estimation of the adhesion potential in Sengupta}
\label{annexe31}
The theoretical adhesion energy considered had five contributions:

\begin{enumerate}
  \item the van der Waals attractive potential given in eq.(\ref{eq_1_VdW}). For simplicity, the last corrective term was omitted;
  \item the gravitational potential given in eq.(\ref{eq_1_grav});
  \item the steric repulsion coming from thermal fluctuations derived by Seifert
    $V_\mathrm{steric}^\mathrm{Seifert}$ given in eq.(\ref{eq_1_Vsteric_Seifert});
  \item a short range steric repulsion coming from the lipids, given by

    \begin{equation}
      V_S = \frac{2 k_\mathrm{B}T}{d_\mathrm{lip}^2} \, e^{-\frac{s}{\ell_\mathrm{ster}}} \, ,
    \end{equation}

    \noindent where $d_\mathrm{lip}$ is the lipid head size and $\ell_\mathrm{ster}$ is the steric repulsion length;
  \item a steric repulsion coming from the polymer coating of the substrate, given by
\begin{equation}
  V_p = \left\{ \begin{array}{ccc} -k_\mathrm{B} T \, c_\mathrm{pol} \ln\left[1 - 2\exp{\left(-\frac{3}{2}\frac{s^2}{R_f^2}\right)}\right]\,\,\, & $for$ &\, s < R_f\, ,\\
    \\
    k_\mathrm{B}T\, c_\mathrm{pol} \left[\frac{1}{2}\ln\left(\frac{3}{8\pi}\frac{s^2}{R_f^2}\right) + \frac{\pi^6}{6}\frac{R_f^2}{s^2}\right] \,\,\,& $for$ &\, s>R_f\, ,\end{array} \right. 
\end{equation}
\noindent where $R_f$ is the Flory radius of the polymer. 
\end{enumerate}
